# Supplementary material for: Three-Dimensional Coherent Diffractive Imaging of Isolated Faceted Nanostructures
Source: arXiv:2208.04044 ancillary file (2022-08-08)
Supplement: Supplementary file 1 [file supplementary.pdf]

# Three-Dimensional Coherent Diffractive Imaging of Isolated Faceted Nanostructures

Supplemental Material

## Edge Analysis

A number $R = 20$ of independent imaging procedures were performed, by randomly initializing the coordinates of the facets. The $20$ reconstruction procedures yield $20$ different spatial distributions of the electronic density $\rho_r(\vec{x})$. From them, the average electronic density $\rho_{avg}(\vec{x})$ was computed. Due to the variations between the different reconstructions $\rho_r(\vec{x})$, the average $\rho_{avg}(\vec{x})$ will no more have an instantaneous transition between sample and vacuum. In particular, for each point on the average reconstruction's edge, the density profile along the line normal to the surface will manifest a *transition width* greater than 0 between vacuum and sample. For this analysis, we define the *transition width* as the length of the transition between $10\%$ and $90\%$ of the average's density profile, as represented in S1. This *transition width* can be computed for each point at the sample's surface, giving a visual overview on the reconstruction's stability.

## The role of constraints

The imaging approach presented in this work heavily relies upon a parametrization of the sample shape, which can be intuitively addressed as *basis set*. This section aims at providing a qualitative intuition about the influence of choosing a suitable basis set for the forward fitting approach.

Fig. S2 compares two fitting results of the same diffraction pattern. The one in Fig. S2a is obtained by using the facets-based description. Instead, the reconstruction in Fig. S2b was performed by describing the shapes as a combination of *spherical harmonics*. Spherical harmonics are a common way to define a function over a sphere, i.e. a function that only depends on the angular coordinates. This *basis set* is highly employed in chemistry, to describe the spatial distribution of atomic orbitals, or in geophysics, to define the *geoid*. Spherical

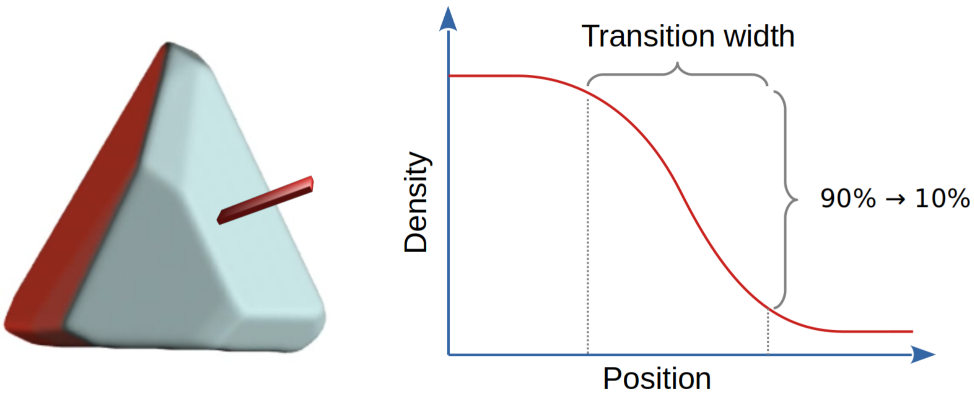


Figure S1: Description of the *edge analysis*. On the left side, a rendering of the average reconstruction is shown, along with a solid line normal to the sample's surface. The sample's density profile computed along that direction is sketched on the right side. The transition width for the given position of the surface is then computed as the length necessary to observe a drop of the average density profile from $90\%$ to $10\%$ of its value.

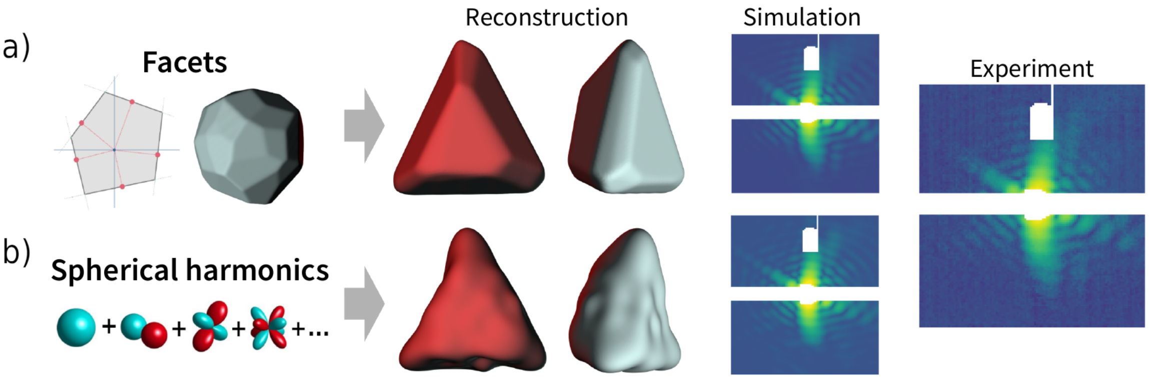


Figure S2: Comparison between reconstructions with different shapes' parametrizations for the same experimental data. In a), the same result presented in Fig. 2e is reported, where the description of the nanocrystal is based on facets. In b) the same diffraction data is fitted with the spherical harmonics basis set. These and others basis sets are provided by the *Scatman* simulation software [1].

harmonics allow to define any shape for which each point of the surface is simply connected to a common center. It is intuitively clear that spherical harmonics are not a convenient basis set for the description of a faceted sample, as a huge number of coefficients is required to accurately describe flat surfaces and edgy vertices. This is well visible in Fig. S2b, where the spherical harmonics expansion was truncated at a degree $l = 8$, to keep the total amount of coefficients at $81$, similar to the amount of spatial parameters involved in the reconstruction of Fig. S2a ($90$, three coordinates for each of the $30$ facets). The overall structures in Fig. S2 are highly comparable, both reporting the same main features of the sample. However, as previously highlighted, Fig. S2b cannot really reproduce well the flat surfaces and the sharp tips, due to the truncation of the spherical harmonics expansion. This directly reflects into the simulated diffraction pattern, whose features are deviating more from the experiment for Fig. S2b (particularly in the lower-right quadrant). The convergence properties of the spherical harmonics reconstruction have still to be investigated, as, in this case, the *convexity* constraint is released. However, such a study goes beyond the scope of this manuscript.

The discussion presented in this section qualitatively shows the strong impact that the choice of the *right* basis set has on the reconstruction quality. Additionally, it implicitly underlines the versatility of our fitting approach, which is completely independent of the employed shape model. This opens exciting possibilities for data analysis of different sample classes, for which different basis sets are more suitable.

# References

[1] Alessandro Colombo, Julian Zimmermann, Bruno Langbehn, Thomas Moller, Christian Peltz, Katharina Sander, Bjorn Kruse, Paul Tummler, Ingo Barke, Daniela Rupp, and Thomas Fennel. The scatman: an approximate method for fast wide-angle scattering simulations, 2022.
